# Supplementary material for: A Unified Picture of Lattice Instabilities in Metallic Transition Metal Dichalcogenides
Source: arXiv:1901.10588 ancillary file (2019-01-29)
Supplement: Supplementary file 1 [file suppl.pdf]

# Supplemental Material for
# "A Unified Picture of Lattice Instabilities in Metallic Transition Metal Dichalcogenides"

Diego Pasquier* and Oleg V. Yazyev†
*Institute of Physics, Ecole Polytechnique Fédérale de Lausanne (EPFL), CH-1015 Lausanne, Switzerland*

## I. COMPUTATIONAL METHODOLOGY

DFT calculations are performed using the QUANTUM ESPRESSO package [1]. We use norm-conserving pseudopotentials from the SG15 library [2–4], that include the $5s$ and $5p$ semicore states of Ta, W and Re explicitly. A plane-wave cutoff of 60 Ry is used. We employ a $24 \times 24$ $k$-point mesh ($12 \times 24$ and $12 \times 12$ for the $2 \times 1$ and $2 \times 2$ supercells, respectively) and a Marzari-Vanderbilt smearing [5] of 10 mRy. We use the cell parameters and atomic positions obtained by relaxing the undoped materials until all the Hellmann-Feynman forces are smaller than $10^{-4}$ Ry/Bohr and the pressure is smaller than 0.1 Kbar. We include about 13 Å of vacuum between periodic replicas. We employ the Wannier90 code [6] to obtain Maximally Localized Wannier Functions (MLWFs). Phonon frequencies are calculated within density functional perturbation theory [7]. To plot the phonon dispersion curves, we have calculated the phonons on a $24 \times 24$ grid of $q$-points and used Fourier interpolation. The susceptibility is evaluated on a $100 \times 100$ $k$-points grid with Wannier-interpolated bands. Doping is simulated by changing the total charge of the electron system, with a compensating jellium backround added to ensure the overall charge neutrality of the unit cell.

## II. WANNIER FUNCTIONS FOR $1T'$-$WS_2$

In the main text, we have discussed the splitting of the $t_{2g}$ states in the $1T'$ phase of single-layer $WS_2$, and presented a plot of one of the two equivalent bonding $t_{2g}$ Wannier functions (WFs). Here, we explain how the MLWFs are constructed and present a few additional plots.

Firstly, we derive MLWFs by including 14 occupied bands and the 2 lowest unoccupied bands. The low-energy sulfur $s$-bands and semicore state bands are excluded. We use the Bloch phases as initial projector and perform the minimization of the spread functional [8]. We obtain 12 $p$-like WFs centered on the sulfur atoms, two $t_{2g}$-like WFs pointing along the chain direction, and two molecular WFs. The molecular WFs are centered on the W–W bonds and clearly resemble bonding combinations of $t_{2g}$ WFs.

Secondly, we wannierize the 6 higher-energy unoccupied bands, obtaining 4 $e_g$-like WFs and 2 antibonding WFs centered on the W–W bonds. Since the bonding and nonbonding $t_{2g}$ WFs in the $1T'$ phase are constructed together with the $p$ WFs, they do not contain explicitly the $pd$ antibonding energy. For proper comparison with the antibonding $t_{2g}$ and $e_g$ WFs, we have therefore added the $t_{2g}$-$p$ hybridization energy of 1.49 eV, calculated according to the methodology proposed in Ref. [9], that we have previously applied to the TMDs in Ref. [10].

Note that in order to obtain the molecular bonding and antibonding WFs centered on the W–W bonds, it is necessary to consider two sets of bands separately, otherwise the maximal localization procedure would yield atomic-like WFs centered on the ions.

Fig. 1(a) shows an isovalue plot of one of the antibonding WFs. Contrary to the bonding WF, the antibonding WF contains some weight on the ligands, which reflects the hybridization with the $3p$ states of sulfur atoms. This difference stems from the fact that the $p$-like bands are excluded when constructing the antibonding $t_{2g}$ and $e_g$ WFs. Fig. 1(b) shows one of the two equivalent nonbonding $t_{2g}$ WF, centered on one of the two W atoms of the unit cell. The nonbonding $t_{2g}$ WFs point along the direction where the W–W distance is unaffected by the distortion compared to the $1T$ phase. The on-site energy of the nonbonding $t_{2g}$ WFs is very close to that of the $t_{2g}$ WFs of the undistorted $1T$ phase. In Fig. 1(c), we present an isovalue plots of one of the four $e_g$-like WFs (two per tungsten atom), with $d_{x^2-y^2}$ character.

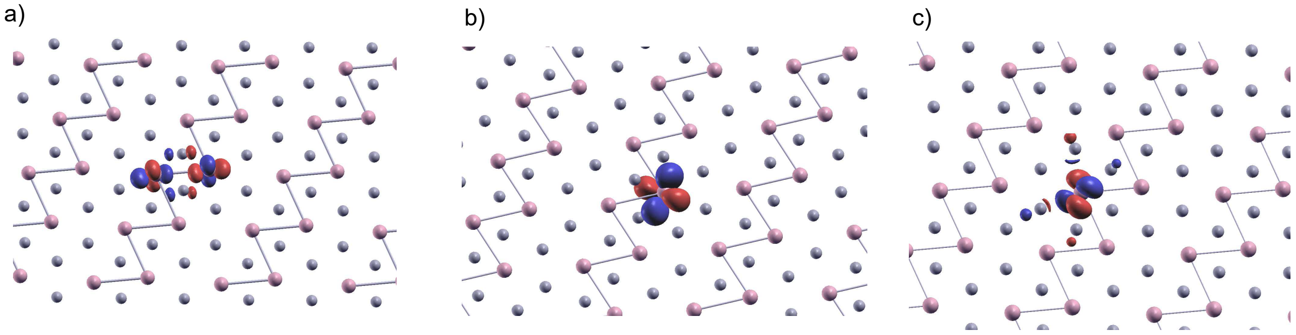


FIG. 1. Selected isovalue plots of Wannier functions (WFs) for monolayer $1T'$-$WS_2$. (a) Antibonding $t_{2g}$ WF. (b) Nonbonding $t_{2g}$ WF. (c) $e_g$ WF with $d_{x^2-y^2}$ character.

## III. WANNIER FUNCTIONS FOR $1T''$-RES$_2$

In the main text, we have discussed the splitting of the $t_{2g}$ subshell of monolayer $ReS_2$ in the $1T''$ phase into six bonding and six antibonding $t_{2g}$ states, and presented a plot of one of the six bonding $t_{2g}$ WFs.

We first consider 30 occupied bands, and obtain 24 $p$-like WFs centered on the 8 sulfur atoms, and 6 bonding $t_{2g}$ WFs, each bond drawn in Fig. 2(a) accomodating one of them. The lower-energy bands, coming from the sulfur $3s$ states and from the transition metal $5s$ and $5p$ semicore states, are excluded.

We then consider 14 unoccupied conduction bands, and obtain the corresponding 6 antibonding $t_{2g}$ WFs, as well as 8 $e_g$ WFs centered on the 4 Re atoms.

In Fig. 2(a), we show an isovalue plot of the corresponding antibonding $t_{2g}$ WF, centered on the same bond. As for $1T'$-$WS_2$, and for the same reasons, the antibonding $t_{2g}$ WFs contain some weight on the sulfur atoms resembling $p$ orbitals. Contrary to the $1T'$ phase of $WS_2$ for which all the W–W bonds are equivalent, the Re–Re bonds in the $1T''$ phase are not all equal. Fig. 2(b) shows another bonding $t_{2g}$ WF, centered on another nonequivalent Re–Re bond. In Fig. 2(c), we show one of the eight $e_g$ WFs, with $d_{z^2}$ orbital character.

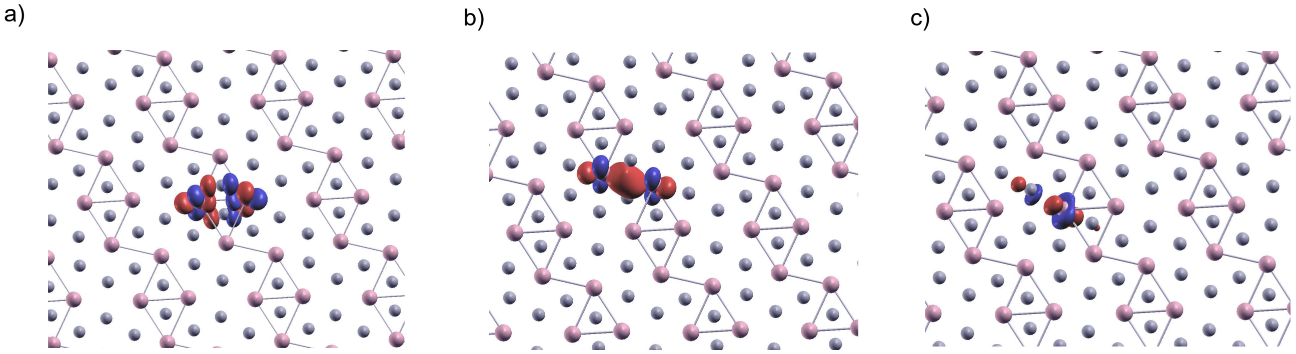


FIG. 2. Selected isovalue plots of Wannier functions (WFs) for monolayer $1T''$-$ReS_2$. (a) Antibonding $t_{2g}$ WF. (b) Bonding $t_{2g}$ WF. (c) $e_g$ WF with $d_{z^2}$ character.

## IV. FERMI SURFACE OF $1T$-WS$_2$

In the main text, we have mentioned the proposed nesting mechanism for the $1T$-to-$1T'$ transition of certain molybdenum dichalcogenides, based on the inspection of the Fermi surface. In Figs. 3(a) and 3(b), we show the Fermi surface of monolayer $1T$-$WS_2$ in the undoped and electron-doped cases (with 0.1 extra electron per formula unit). One can see that in the electron-doped case, some extra small electron pockets are present. These pockets are approximately nested by the vector $\Gamma M$. However, the absence of these pockets in the undoped case shows that the instability at the $M$ point is not related to them. The mechanism for the $1T$-to-$1T'$ instability in the $d^2$ TMDs must be universal, so the nesting of these pockets cannot account for the distortion in the Mo dichalcogenides either.

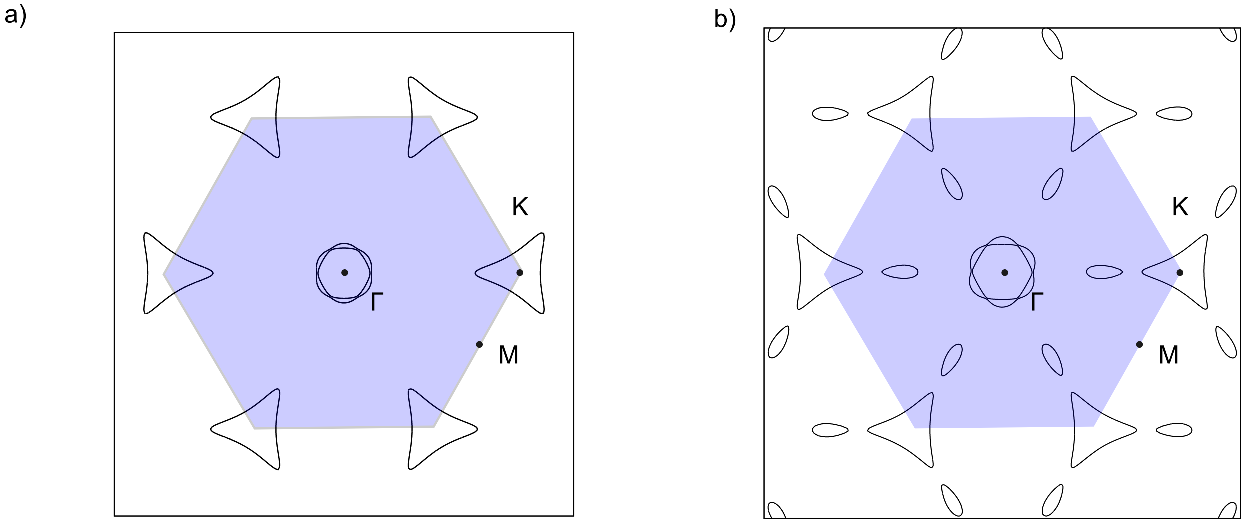


FIG. 3. Fermi surface for monolayer 1$T$-$WS_2$ for the (a) undoped, and (b) electron-doped (+0.1 electron per formula unit) cases. The shaded areas indicate the Brillouin zone.

* diego.pasquier@epfl.ch
† oleg.yazyev@epfl.ch

[1] Giannozzi *et al.*, J. Phys.: Condens. Matter **21**, 395502 (2009).
[2] D. R. Hamann, Phys. Rev. B **88**, 085117 (2013).
[3] P. Scherpelz, M. Govoni, I. Hamada, and G. Galli, J. Chem. Theory Comput. **12**, 3523 (2016).
[4] `http://www.quantum-simulation.org/potentials/sg15_oncv/`.
[5] N. Marzari, D. Vanderbilt, A. De Vita, and M. C. Payne, Phys. Rev. Lett. **82**, 3296 (1999).
[6] A. A. Mostofi, J. R. Yates, G. Pizzi, Y.-S. Lee, I. Souza, D. Vanderbilt, and N. Marzari, Comput. Phys. Commun. **185**, 2309 (2014).
[7] S. Baroni, S. de Gironcoli, A. Dal Corso, and P. Giannozzi, Rev. Mod. Phys. **73**, 515 (2001).
[8] N. Marzari and D. Vanderbilt, Phys. Rev. B **56**, 12847 (1997).
[9] A. Scaramucci, J. Ammann, N. Spaldin, and C. Ederer, J. Phys.: Condens. Matter **27**, 175503 (2015).
[10] D. Pasquier and O. V. Yazyev, arXiv:1810.01302 (2018).
